# Supplementary material for: Visualizing Bags of Vectors
Source: arXiv:1310.3333 source file (2013-10-12)
Supplement: Supplementary file 1 [file HAT-Supplementary-Notes.pdf]

# Heirarchical Author Topic Model

## Supplementary Notes

Raghuram Reddy Nagireddy
rrn2111@columbia.edu

Sriramkumar Balasubramanian
sb3457@columbia.edu

**Notation:**

$l$ - total number of levels in the heirarchy
$t_k$ - a possible topic at level k
$z_{i,j}$ - topic assigned to a word i at level j
$\boldsymbol{\theta_{j<l}}$ - random variable denoting the distribution of topics (categorical) at level j conditioned on the topics at level j-1 with an exception for j=1 when $\theta$ becomes unconditional
$\boldsymbol{\theta\prime_k}$ - random variable denoting the distribution of topics (categorical) for author k at level l(the leaf level)
$\theta_{j,t_j,t_{j-1}}$ - probability of topic $t_j$ at level j conditioned on topic $t_{j-1}$ at level j-1
$\theta\prime_{k,t_l,t_{l-1}}$ - probability of topic $t_l$ at level l conditioned on topic $t_{l-1}$ at level l-1
$\boldsymbol{\alpha_j}$ - Dirichlet prior parameter for $\boldsymbol{\theta_{j<l}}$
$\boldsymbol{\alpha\prime_k}$ - Dirichlet prior parameter for $\boldsymbol{\theta\prime_k}$
$\boldsymbol{\phi}$ - random variable denoting the word distributions of a topic in level l (last or the leaf level)
$n_{j,t_j,t_{j-1}}$ - number of times topic $t_j$ at level j is assigned together with topic $t_{j-1}$ at level j-1
$n\prime_{k,t_l,t_{l-1}}$ - number of times topic $t_l$ at level l is assigned together with topic $t_{l-1}$ at level l-1 for an author k
$\phi_{t,w}$ - probability that a word w is generated by topic t from the leaf level
$\prod_v$ - denotes the product taken over all possible enumerations of v in its domain
** All other variables that are common to the Author-Topic model and are not included here

**Assumptions:**

We assume in the model that,
1. Only the leaf level topics generate words, in other words $\phi_{t,w}$ depends only the **leaf** level topic t apart from the word w
2. In accordance with the graphical model we propose, we assume that the topics conditioned on their parent topics are generated independent of authors
3. An author is responsible for generating only a leaf topic
4. Conditioned on a topic the distribution of a word is independent of the author for that word (same as in AT model)

**Gibbs Sampler for Heirarchical Author-Topic Model:**

We need to compute $P(\mathbf{z_i} = (t_1, t_2..t_l), x_i = k|\mathbf{z_{-i}}, \mathbf{w}, \mathbf{x_{-i}}, \mathbf{a_d})$ for the Gibbs Sampler iterations.
This is $\propto P(\mathbf{z_i} = (t_1, t_2..t_l), x_i = k, \mathbf{z_{-i}}, \mathbf{w}, \mathbf{x_{-i}}, \mathbf{a_d}; \alpha, \beta)$.

This boils down to finding structural form for the total probability, $P(\mathbf{z},\mathbf{x},\mathbf{w};\alpha,\beta)$

$$= \int_{\phi} P(\mathbf{w}|\mathbf{z},\phi)P(\phi;\beta)d\phi \int_{\theta} P(\mathbf{z}|\mathbf{x},\theta)P(\theta;\alpha)d\theta$$

We shall now derive a closed form expression for this in terms of various counts of words and topics. Consider the second integral:

$$= \int_{\boldsymbol{\theta}} \prod_i P(\boldsymbol{z_i}|\boldsymbol{x_i},\boldsymbol{\theta})P(\boldsymbol{\theta};\boldsymbol{\alpha})d\boldsymbol{\theta}$$

$$= \int_{\boldsymbol{\theta}} \prod_i \prod_{j<l} P(z_{i,j}|z_{i,j-1},\boldsymbol{\theta})P(z_{i,l}|z_{i,l-1},\boldsymbol{x_i},\boldsymbol{\theta})P(\boldsymbol{\theta};\boldsymbol{\alpha})d\boldsymbol{\theta}$$

$$= \int_{\boldsymbol{\theta}} \prod_{j<l} \left[ \frac{\Gamma(\sum_{t_j,t_{j-1}} \alpha_{j,t_j,t_{j-1}})}{\prod_{t_j,t_{j-1}} \Gamma(\alpha_{j,t_j,t_{j-1}})} \prod_{t_j,t_{j-1}} \theta_{j,t_j,t_{j-1}}^{\alpha_{j,t_j,t_{j-1}}-1} \prod_{t_j,t_{j-1}} \theta_{j,t_j,t_{j-1}}^{n_{j,t_j,t_{j-1}}} \right] d\boldsymbol{\theta}\times$$

$$\prod_k \int_{\boldsymbol{\theta_k}} \left[ \frac{\Gamma(\sum_{t_l,t_{l-1}} \alpha\prime_{k,t_l,t_{l-1}})}{\prod_{t_l,t_{l-1}} \Gamma(\alpha\prime_{k,t_l,t_{l-1}})} \prod_{t_l,t_{l-1}} \theta\prime_{k,t_l,t_{l-1}}^{\alpha\prime_{k,t_l,t_{l-1}}-1} \prod_{t_l,t_{l-1}} \theta\prime_{k,t_l,t_{l-1}}^{n\prime_{k,t_l,t_{l-1}}} \right] d\boldsymbol{\theta_k}$$

$$= \int_{\boldsymbol{\theta}} \prod_{j<l} \left[ \frac{\Gamma(\sum_{t_j,t_{j-1}} \alpha_{j,t_j,t_{j-1}})}{\prod_{t_j,t_{j-1}} \Gamma(\alpha_{j,t_j,t_{j-1}})} \prod_{t_j,t_{j-1}} \theta_{j,t_j,t_{j-1}}^{\alpha_{j,t_j,t_{j-1}}+n_{j,t_j,t_{j-1}}-1} \right] d\boldsymbol{\theta}\times$$

$$\prod_k \int_{\boldsymbol{\theta_k}} \left[ \frac{\Gamma(\sum_{t_l,t_{l-1}} \alpha\prime_{k,t_l,t_{l-1}})}{\prod_{t_l,t_{l-1}} \Gamma(\alpha\prime_{k,t_l,t_{l-1}})} \prod_{t_l,t_{l-1}} \theta\prime_{k,t_l,t_{l-1}}^{\alpha\prime_{k,t_l,t_{l-1}}+n\prime_{k,t_l,t_{l-1}}-1} \right] d\boldsymbol{\theta_k}$$

Using the following integrals:

$$\int_{\boldsymbol{\theta_k}} \frac{\Gamma(\sum_{t_j,t_{j-1}} \alpha_{j,t_j,t_{j-1}} + n_{k,j,t_j,t_{j-1}})}{\prod_{t_j,t_{j-1}} \Gamma(\alpha_{j,t_j,t_{j-1}} + n_{k,j,t_j,t_{j-1}})} \prod_{t_j,t_{j-1}} \theta_{k,j,t_j,t_{j-1}}^{\alpha_{j,t_j,t_{j-1}}+n_{k,j,t_j,t_{j-1}}-1} d\boldsymbol{\theta_k} = 1$$

$$\int_{\boldsymbol{\theta}} \frac{\Gamma(\sum_{t_j,t_{j-1}} \alpha_{j,t_j,t_{j-1}} + n_{j,t_j,t_{j-1}})}{\prod_{t_j,t_{j-1}} \Gamma(\alpha_{j,t_j,t_{j-1}} + n_{j,t_j,t_{j-1}})} \prod_{t_j,t_{j-1}} \theta_{j,t_j,t_{j-1}}^{\alpha_{j,t_j,t_{j-1}}+n_{j,t_j,t_{j-1}}-1} d\boldsymbol{\theta} = 1$$

The above expression evaluates to,

$$\prod_{j<l} \frac{\Gamma(\sum_{t_j,t_{j-1}} \alpha_{j,t_j,t_{j-1}})}{\prod_{t_j,t_{j-1}} \Gamma(\alpha_{j,t_j,t_{j-1}})} \frac{\prod_{t_j,t_{j-1}} \Gamma(\alpha_{j,t_j,t_{j-1}} + n_{j,t_j,t_{j-1}})}{\Gamma(\sum_{t_j,t_{j-1}} \alpha_{j,t_j,t_{j-1}} + n_{j,t_j,t_{j-1}})} \prod_k \frac{\Gamma(\sum_{t_l,t_{l-1}} \alpha\prime_{k,t_l,t_{l-1}})}{\prod_{t_l,t_{l-1}} \Gamma(\alpha\prime_{k,t_l,t_{l-1}})} \frac{\prod_{t_l,t_{l-1}} \Gamma(\alpha\prime_{k,t_l,t_{l-1}} + n\prime_{k,t_l,t_{l-1}})}{\Gamma(\sum_{t_l,t_{l-1}} \alpha\prime_{k,t_l,t_{l-1}} + n\prime_{k,t_l,t_{l-1}})}$$

Now, the first integral is trivial by observing that (by assumption),

$$P(w|\mathbf{z_i} = (t_1, t_2..t_l)) = P(w|z_{i,l} = t_l)$$

Looking at this expression, it is easy to see that,

$$p(\boldsymbol{z_i}, x_i = k|\boldsymbol{z_{-i}}, \boldsymbol{x_{-i}}, \boldsymbol{w_{-i}}, w_i = m) \propto$$

$$\prod_{j<l}\left[\frac{n_{j,t_j,t_{j-1}}+\alpha_{k,j,t_j,t_{j-1}}}{\sum_{t_j} n_{j,t_j,t_{j-1}}+\alpha_{k,j,t_j,t_{j-1}}}\right]\prod_{k}\left[\frac{n\prime_{k,t_l,t_{l-1}}+\alpha\prime_{k,t_l,t_{l-1}}}{\sum_{t_l} n\prime_{k,t_l,t_{l-1}}+\alpha\prime_{k,t_l,t_{l-1}}}\right]\frac{N_{m,t_l}+\beta}{\sum_{m'} N_{m',t_l}+\beta}$$

Note that using the above expression we can only generate the samples from the joint distribution $p(\boldsymbol{z_i}, x_i = k)$. Instead we propose to perform Gibbs Sampling over this joint as well by sampling each component of z as follows:

$$p(z_{i,j} = t_j|\boldsymbol{z_{-i}}, z_{i,j-1} = t_{j-1}, \boldsymbol{x_{-i}}, \boldsymbol{w_{-i}}, w_i = m) \propto$$
$$\frac{n_{j,t_j,t_{j-1}}+\alpha_{j,t_j,t_{j-1}}}{\sum_{t_j} n_{j,t_j,t_{j-1}}+\alpha_{j,t_j,t_{j-1}}}\frac{n_{j+1,t_{j+1},t_j}+\alpha_{j+1,t_{j+1},t_j}}{\sum_{t_{j+1}} n_{j+1,t_{j+1},t_j}+\alpha_{j+1,t_{j+1},t_j}}$$

, for j<l

For the leaf topics,

$$p(z_{i,l} = t_l, x_i = k|\boldsymbol{z_{-i}}, z_{i,l-1} = t_{l-1}, \boldsymbol{x_{-i}}, \boldsymbol{w_{-i}}, w_i = m) \propto$$
$$\frac{n\prime_{k,t_l,t_{l-1}}+\alpha\prime_{k,t_l,t_{l-1}}}{\sum_{t_l} n\prime_{k,t_l,t_{l-1}}+\alpha\prime_{k,t_l,t_{l-1}}}\frac{N_{m,t_l}+\beta}{\sum_{m'} N_{m',t_l}+\beta}$$
